# Supplementary material for: Universal Shape Replicators via Self-Assembly with Attractive and Repulsive Forces
Source: arXiv:1608.00477 source file (2016-08-01)
Supplement: Supplementary file 1 [file appendix.tex]

\section{Glue Strength Details}\label{sec:glueStrengthInequalities}
Table~\ref{tbl:inequalities} shows the set of glue strength inequalities which must be satisfied for the construction to function.

\input{detachCheck.tex}

%\section{Omitted Construction Details}

%\subsection{Outer Mold Corner Gadgets}\label{sec:app:outercorner}
% outer mold corner

%\FloatBarrier
%\subsection{Outer Drill Corner Gadgets}\label{sec:app:outerdrillcorner}
% outer drill acute corner

%\FloatBarrier
%\subsection{Inner Mold Corner Gadgets}
% inner drill obtuse

%\FloatBarrier
%\subsection{Inner Drill Gadgets}
